# Supplementary material for: Sparse Views, Near Light: A Practical Paradigm for Uncalibrated Point-light Photometric Stereo
Source: arXiv:2404.00098 source file (2024-03-29)
Supplement: Supplementary file 1 [file 02_additional_real_world.tex]

\begin{figure}[t]
  \centering
  \small
  \newcommand{\mywidthc}{0.02\textwidth}
  \newcommand{\mywidthx}{0.48\textwidth}
  \newcolumntype{C}{ >{\centering\arraybackslash} m{\mywidthc} }
  \newcolumntype{X}{ >{\centering\arraybackslash} m{\mywidthx} }
  \newcommand{\tabelt}[1]{\hfil\hbox to 0pt{\hss #1 \hss}\hfil}
  \setlength\tabcolsep{2pt} %
\vspace{-3.5mm}
\begin{subfigure}{0.3\linewidth}
\begin{tabular}{l|cc|}
~ & psnerf & ours\\
\cline{1-3}
& &\\[-3.5mm]
\bear & 8.8 & \textbf{3.5}\\
\buddha & 13.9 & \textbf{10.8}\\
\pot & 9.2 & \textbf{5.1}\\
\reading & 11.9 & \textbf{7.1}\\
\cow & 8.9 & \textbf{3.6}
\end{tabular}
\caption{MAE on diligent.}
\label{tab:diligent}
\end{subfigure}
\hspace{5mm}
\begin{subfigure}{0.5\linewidth}
  \begin{tabular}{XX}
  \includegraphics[width=\mywidthx]{images/rebuttal/real_birds/input_flamingo.png} &
    \includegraphics[width=\mywidthx]{images/rebuttal/real_birds/output_flamingo.png}\\
    \includegraphics[width=\mywidthx]{images/rebuttal/real_birds/input_hawk.png} & \includegraphics[width=\mywidthx]{images/rebuttal/real_birds/output_hawk.png}
  \end{tabular}
  \vspace{-1.0mm}
  \caption{Two scans captured ourself.}
  \label{fig:real_birds}
  \end{subfigure}
\vspace{-3.0mm}
\caption{Seven additional real-world experiments}
\label{fig:additional_real_world}
\end{figure}
